# Supplementary material for: The Case for Learning Application Behavior to Improve Hardware Energy Efficiency
Source: arXiv:2004.13074 source file (2020-11-23)
Supplement: Supplementary file 1 [file appendix.tex]

\subsection{Updated Hardware Implementation}
\subsubsection{DNN Driver Module Structure}

\subsubsection{Hardware Overhead}

\subsection{Forecaster with Larger Input}
